# Supplementary material for: Digital Histopathology with Graph Neural Networks: Concepts and Explanations for Clinicians
Source: arXiv:2312.02225 source file (2023-12-28)
Supplement: Supplementary file 1 [file appendix.tex]

\chapter{Software Licenses}
