# Supplementary material for: Digital Histopathology with Graph Neural Networks: Concepts and Explanations for Clinicians
Source: arXiv:2312.02225 source file (2023-12-28)
Supplement: Supplementary file 2 [file appendix_old.tex]

\chapter{TO BE RENAMED}

%TODO GET PROOF READ
\section{Properties of Absorbance}
\begin{definition}[\textbf{Absorbance}] For a block of material m, the absorbance is
\begin{equation}
    A(m) \triangleq -log(\frac{I_t}{I_r})
\end{equation}
where $I_t$ and $I_r$ is the radiance transmitted and received by the material. 
\begin{figure}[H]
    \centering
    \includegraphics[width=8cm,height=6cm,keepaspectratio]{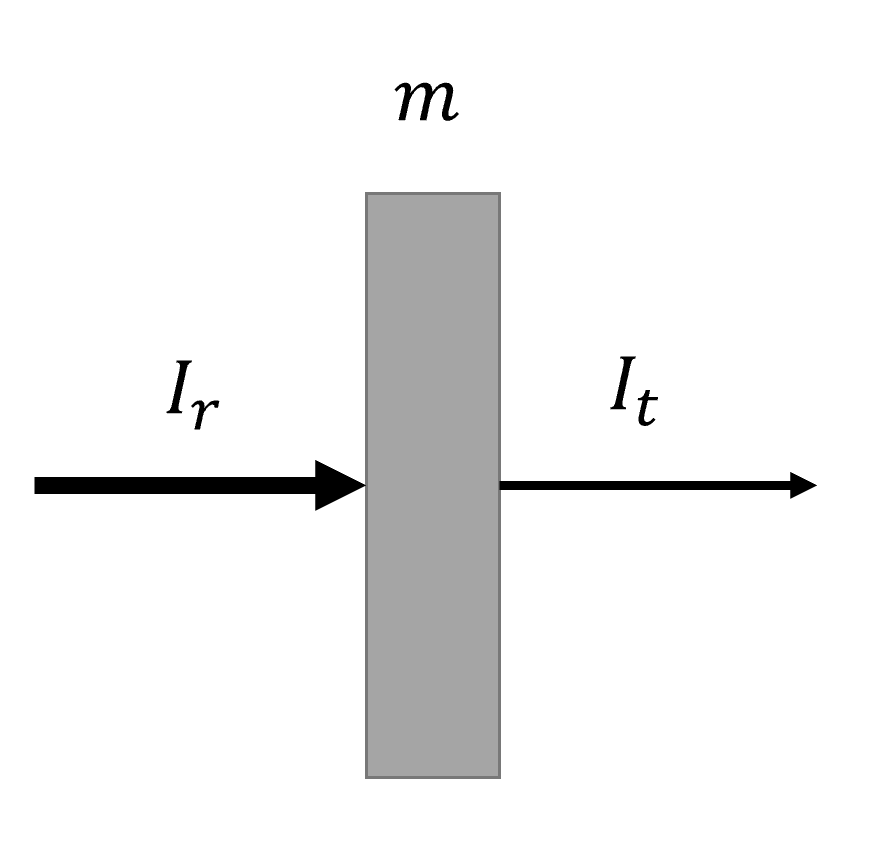}
    \caption{A block of material `m' with light passing through}
    \label{fig:absorbance_def}
\end{figure}
Note, the absorbance of no material is 0 ($A(0)=-log(\frac{I_r}{I_r})=0$) and the addition of two blocks corresponds to stacking them one on top of eachother.
\end{definition}
\begin{lemma}[\textbf{Linearity of Absorbance}]
\label{lemma:linearity_of_absorbance}
Absorbance of a composition is a linear combination of the constituents' absorbance. I.e. for materials $a$\&$b$, and scalar $\lambda$
\begin{equation}    
    A(a+b) = A(a) + A(b)
\end{equation} 
\begin{equation}
    A({\lambda a}) = \lambda A(a)
\end{equation}   
\end{lemma}
\begin{proof} 
Firstly, linearity under addition:
\begin{figure}[H]
    \centering
    \includegraphics[width=8cm,height=6cm,keepaspectratio]{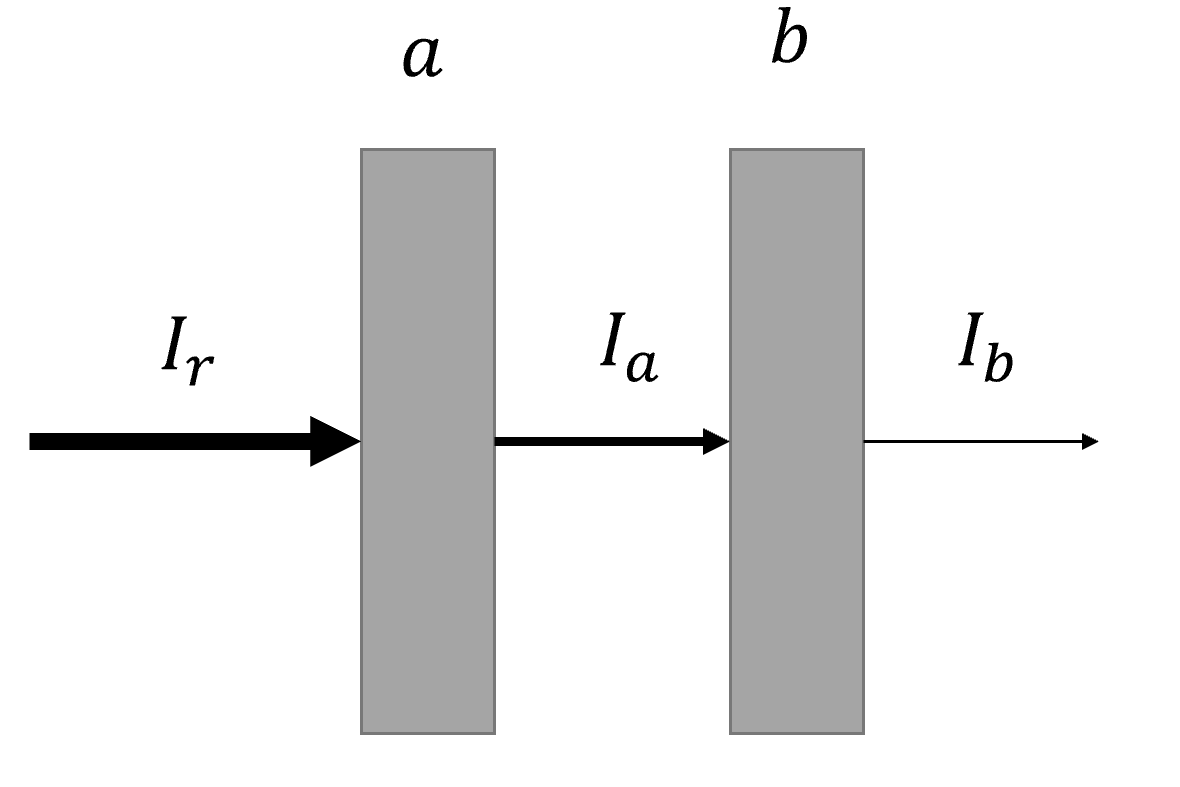}
    \caption{Block of material `a' stacked on block of material `b'}
    \label{fig:add_linear_abs}
\end{figure}
\begin{align*}
    A(a)+A(b) & = -log(\frac{I_a}{I_r}) + -log(\frac{I_b}{I_a}) \\ &  = -log(\frac{I_b}{I_r})
    \\ & = A(a+b)
\end{align*}
Secondly, a rough sketch of linearity under scalar multiplication:
\begin{figure}[H]
    \centering
    \includegraphics[width=8cm,height=6cm,keepaspectratio]{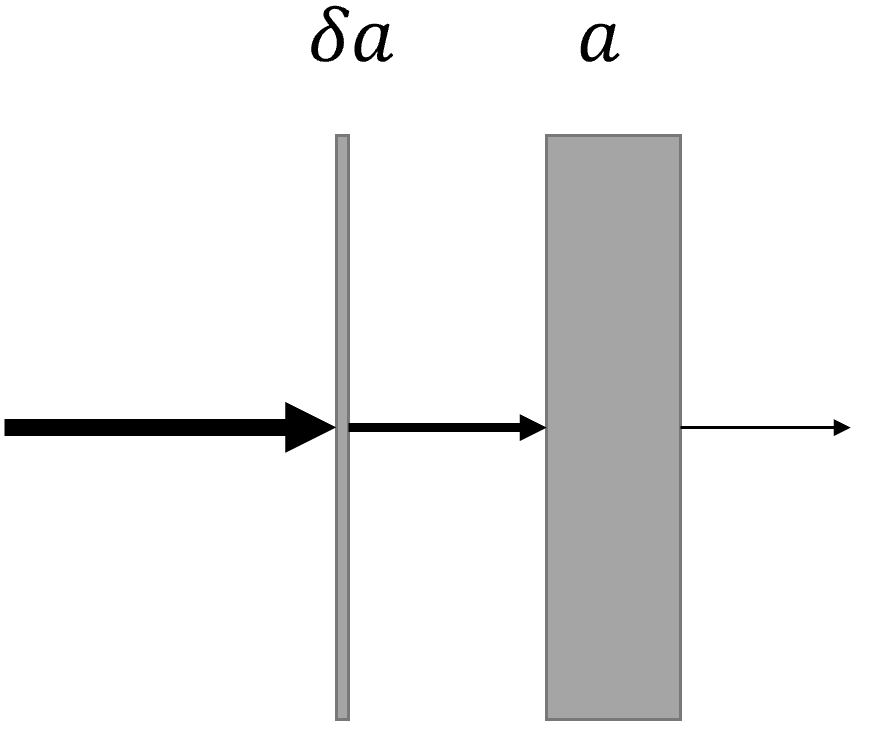}
    \caption{a thin vernier on top of block `a' of same material}
    \label{fig:mult_linear_abs}
\end{figure}
By linearity of addition, $A(a+ \delta a) = A(a)+A(\delta a)$. Taylor approximation of $A(\delta a)$ to first order is $A(0) + \delta a A'(0) = \delta a A'(0)$. This implies:
\begin{align*}
    A(a+\delta a) & = A(a) + \delta a A'(0) \\
    \frac{A(a + \delta a) - A(a)}{\delta a} & = A'(0) \\
    A'(a) & = A'(0) = c \\
    \implies A(x) & = cx
\end{align*}
For a constant c. Hence, by stacking enough verniers to get a block of material a and thickness $\lambda$, 
$$A(\lambda a) = c \lambda a = \lambda c a = \lambda A(a)$$
\end{proof}

%TODO IMRPOVE CLARITY - Consider naming blocks one thing and material other.


\chapter{Machine Learning Theory Expanded}

\begin{algorithm}[H]
\caption{Gradient descent}\label{alg:dl_learn}
\begin{algorithmic}[1]

\State $w \gets$ initial weights.
\For{$t$ steps}
    \State $\hat{Y} \gets f(X;w)$
    \State $loss \gets E(\hat{Y},Y)$
    \State $w \gets w - \alpha \nabla_w loss$   \Comment{Optimization step}
\EndFor
\end{algorithmic}
\end{algorithm}

%TAble of neural network layers and the associate functions they compute
